# Supplementary material for: Ab-initio calculations of carbon and boron nitride allotropes and their structural phase transitions using periodic coupled cluster theory
Source: arXiv:1902.08100 source file (2019-02-21)
Supplement: Supplementary file 1 [file supp.pdf]

# Supplementary Information: “$Ab-initio$ calculations of carbon and boron nitride allotropes and their structural phase transitions using periodic coupled cluster theory”

Thomas Gruber[1] and Andreas Grüneis[1, 2, *]

[1] *Max-Planck-Institute for Solid State Research, Heisenbergstraße 1, 70569 Stuttgart, Germany*
[2] *Institute for Theoretical Physics, Vienna University of Technology, Wiedner Hauptstrasse 8-10, 1040 Vienna, Austria*

(Dated: September 21, 2018)

* andreas.grueneis@tuwien.ac.at

TABLE I. Structural parameters of BN-bw-TS. All units in [Å]. Atomic positions in fractional coordinates. See article for further details.

| | | | |
|---|---|---|---|
| $\vert\vec{a}\vert$ | 2.5108346939 | 0.0000000000 | 0.0000000000 |
| $\vert\vec{b}\vert$ | 0.0000000000 | 4.2192764282 | 0.0000000000 |
| $\vert\vec{c}\vert$ | 0.0000000000 | 0.0000000000 | 4.8998184204 |
| Boron | 0 | 0 | 0 |
| Boron | 0.5 | 0.5 | 0.08562 |
| Boron | 0 | 0.50005 | 0.58562 |
| Boron | 0.5 | 0 | 0.5 |
| Nitrogen | 0 | 0.84926 | 0.58562 |
| Nitrogen | 0.5 | 0.34926 | 0.5 |
| Nitrogen | 0.5 | 0.84922 | 0.08562 |
| Nitrogen | 0 | 0.34922 | 0 |

TABLE II. Structural parameters of BN-l-pc-TS. All units in [Å]. Atomic positions in fractional coordinates. See article for further details.

| | | | |
|---|---|---|---|
| $\vert\vec{a}\vert$ | 2.5130965710 | 0.0000000000 | 0.0000000000 |
| $\vert\vec{b}\vert$ | 0.0000000000 | 4.2820081711 | 0.0000000000 |
| $\vert\vec{c}\vert$ | 0.0000000000 | 0.8552707585 | 4.6290988549 |
| Boron | 0.5 | 0.4834 | 0.08643 |
| Boron | 0 | 0.4834 | 0.58643 |
| Boron | 0.5 | 0 | 0.5 |
| Boron | 0 | 0 | 0 |
| Nitrogen | 0.5 | 0.3558 | 0.43973 |
| Nitrogen | 0.5 | 0.83936 | 0.02616 |
| Nitrogen | 0 | 0.83936 | 0.52616 |
| Nitrogen | 0 | 0.3558 | 0.93973 |

TABLE III. Structural parameters of BN-pc-TS. All units in [Å]. Atomic positions in fractional coordinates. See article for further details.

| | | | |
|---|---|---|---|
| $\vert\vec{a}\vert$ | 2.50612000 | 0.00000000 | 0.00000000 |
| $\vert\vec{b}\vert$ | 0.00000000 | 4.34072717 | 0.00000000 |
| $\vert\vec{c}\vert$ | 0.00000000 | 1.44691071 | 4.71446633 |
| Boron | 0.5 | 0 | 0.5 |
| Boron | 0 | 0 | 0 |
| Boron | 0 | 0.5 | 0.5 |
| Boron | 0.5 | 0.5 | 0 |
| Nitrogen | 0.000001 | 0.85238 | 0.44287 |
| Nitrogen | 0.5 | 0.85238 | 0.94287 |
| Nitrogen | 0.500001 | 0.35238 | 0.44287 |
| Nitrogen | 0 | 0.35238 | 0.94287 |

TABLE IV. Structural parameters of BN-pw-TS. All units in [Å]. Atomic positions in fractional coordinates. See article for further details.

| | | | |
|---|---|---|---|
| $\|\vec{a}\|$ | 2.50606000 | 0.00000000 | 0.00000000 |
| $\|\vec{b}\|$ | 0.00000000 | 4.34062281 | 0.00000000 |
| $\|\vec{c}\|$ | 0.00000000 | 0.00000000 | 4.74221000 |
| Boron | 0 | 0 | 0 |
| Boron | 0.5 | 0.833333 | 0.500001 |
| Boron | 0.5 | 0.5 | 0 |
| Boron | 0 | 0.3333333333 | 0.500001 |
| Nitrogen | 0 | 0 | 0.443245 |
| Nitrogen | 0.5 | 0.833333 | 0.943244 |
| Nitrogen | 0.5 | 0.5 | 0.443245 |
| Nitrogen | 0 | 0.3333333333 | 0.943244 |

TABLE V. Structural parameters of $r$-BN. All units in [Å]. Atomic positions in fractional coordinates. See article for further details.

| | | | |
|---|---|---|---|
| $\|\vec{a}\|$ | 2.48778000 | 0.00000000 | 0.00000000 |
| $\|\vec{b}\|$ | 0.00000000 | 4.30896266 | 0.00000000 |
| $\|\vec{c}\|$ | 0.00000000 | 1.43631949 | 6.45855008 |
| Boron | 0 | 0 | 0 |
| Boron | 0.5 | 0 | 0.5 |
| Boron | 0.5 | 0.5 | 0 |
| Boron | 0 | 0.5 | 0.5 |
| Nitrogen | 0.5 | 0.8333333333 | 0 |
| Nitrogen | 0 | 0.8333333333 | 0.5 |
| Nitrogen | 0 | 0.3333333333 | 0 |
| Nitrogen | 0.5 | 0.3333333333 | 0.5 |

TABLE VI. Structural parameters of BN-AB. All units in [Å]. Atomic positions in fractional coordinates. See article for further details.

| | | | |
|---|---|---|---|
| $\|\vec{a}\|$ | 2.48776000 | 0.00000000 | 0.00000000 |
| $\|\vec{b}\|$ | 0.00000000 | 4.30892715 | 0.00000000 |
| $\|\vec{c}\|$ | 0.00000000 | 0.00000000 | 6.45794000 |
| Boron | 0 | 0 | 0 |
| Boron | 0.5 | 0.1666666667 | 0.5 |
| Boron | 0.5 | 0.5 | 0 |
| Boron | 0 | 0.6666666667 | 0.5 |
| Nitrogen | 0 | 0 | 0.5 |
| Nitrogen | 0 | 0.3333333333 | 0 |
| Nitrogen | 0.5 | 0.5 | 0.5 |
| Nitrogen | 0.5 | 0.8333333333 | 0 |

TABLE VII. Structural parameters of $h$-BN. All units in [Å]. Atomic positions in fractional coordinates. See article for further details.

| | | | |
|---|---|---|---|
| $\vert\vec{a}\vert$ | 2.48813000 | 0.00000000 | 0.00000000 |
| $\vert\vec{b}\vert$ | 0.00000000 | 4.30956758 | 0.00000000 |
| $\vert\vec{c}\vert$ | 0.00000000 | 0.00000000 | 6.49122000 |
| Boron | 0.5 | 0.5 | 0 |
| Boron | 0 | 0.3333333333 | 0.5 |
| Boron | 0 | 0 | 0 |
| Boron | 0.5 | 0.8333333333 | 0.5 |
| Nitrogen | 0.5 | 0.5 | 0.5 |
| Nitrogen | 0 | 0.3333333333 | 0 |
| Nitrogen | 0 | 0 | 0.5 |
| Nitrogen | 0.5 | 0.8333333333 | 0 |

TABLE VIII. Structural parameters of $c$-BN. All units in [Å]. Atomic positions in fractional coordinates. See article for further details.

| | | | |
|---|---|---|---|
| $\vert\vec{a}\vert$ | 2.53240000 | 0.00000000 | 0.00000000 |
| $\vert\vec{b}\vert$ | 0.00000000 | 4.38624547 | 0.00000000 |
| $\vert\vec{c}\vert$ | 0.00000000 | 1.46208564 | 4.13539053 |
| Boron | 0.5 | 0 | 0.5 |
| Boron | 0 | 0 | 0 |
| Boron | 0 | 0.5 | 0.5 |
| Boron | 0.5 | 0.5 | 0 |
| Nitrogen | 0 | 0.875 | 0.375 |
| Nitrogen | 0.5 | 0.875 | 0.875 |
| Nitrogen | 0.5 | 0.375 | 0.375 |
| Nitrogen | 0 | 0.375 | 0.875 |

TABLE IX. Structural parameters of $w$-BN. All units in [Å]. Atomic positions in fractional coordinates. See article for further details.

| | | | |
|---|---|---|---|
| $\vert\vec{a}\vert$ | 2.52377000 | 0.00000000 | 0.00000000 |
| $\vert\vec{b}\vert$ | 0.00000000 | 4.37129875 | 0.00000000 |
| $\vert\vec{c}\vert$ | 0.00000000 | 0.00000000 | 4.17603000 |
| Boron | 0 | 0 | 0 |
| Boron | 0.5 | 0.8333333333 | 0.5 |
| Boron | 0.5 | 0.5 | 0 |
| Boron | 0 | 0.333333 | 0.5 |
| Nitrogen | 0 | 0 | 0.374462 |
| Nitrogen | 0.5 | 0.8333333333 | 0.874462 |
| Nitrogen | 0.5 | 0.5 | 0.374462 |
| Nitrogen | 0 | 0.333333 | 0.874462 |

TABLE X. Structural parameters of C-bw-TS. All units in [Å]. Atomic positions in fractional coordinates. See article for further details.

| | | | |
|---|---|---|---|
| $\|\vec{a}\|$ | 2.4713423252 | 0.0000000000 | 0.0000000000 |
| $\|\vec{b}\|$ | 0.0000000000 | 4.1638784409 | 0.0000000000 |
| $\|\vec{c}\|$ | 0.0000000000 | 0.0000000000 | 4.8353328705 |
| Carbon | 0 | 0 | 0 |
| Carbon | 0.5 | 0.5 | 0.08562 |
| Carbon | 0 | 0.5 | 0.58562 |
| Carbon | 0.5 | 0 | 0.5 |
| Carbon | 0 | 0.84924 | 0.58562 |
| Carbon | 0.5 | 0.34924 | 0.5 |
| Carbon | 0.5 | 0.84924 | 0.08562 |
| Carbon | 0 | 0.34924 | 0 |

TABLE XI. Structural parameters of C-l-pc-TS. All units in [Å]. Atomic positions in fractional coordinates. See article for further details.

| | | | |
|---|---|---|---|
| $\|\vec{a}\|$ | 2.4561738968 | 0.0000000000 | 0.0000000000 |
| $\|\vec{b}\|$ | 0.0000000000 | 4.2290029526 | 0.0000000000 |
| $\|\vec{c}\|$ | 0.0000000000 | 0.7924479049 | 4.6373511739 |
| Carbon | 0.5 | 0 | 0.5 |
| Carbon | 0.5 | 0.35692 | 0.4414 |
| Carbon | 0.5 | 0.48174 | 0.08868 |
| Carbon | 0 | 0 | 0 |
| Carbon | 0 | 0.35692 | 0.9414 |
| Carbon | 0 | 0.48174 | 0.58868 |
| Carbon | 0 | 0.83866 | 0.53008 |
| Carbon | 0.5 | 0.83866 | 0.03008 |

TABLE XII. Structural parameters of C-pc-TS. All units in [Å]. Atomic positions in fractional coordinates. See article for further details.

| | | | |
|---|---|---|---|
| $\|\vec{a}\|$ | 2.46503000 | 0.00000000 | 0.00000000 |
| $\|\vec{b}\|$ | 0.00000000 | 4.26955720 | 0.00000000 |
| $\|\vec{c}\|$ | 0.00000000 | 1.42317995 | 4.68788848 |
| Carbon | 0.5 | 0.85365 | 0.93904 |
| Carbon | 0 | 0.85365 | 0.43904 |
| Carbon | 0 | 0 | 0 |
| Carbon | 0.5 | 0 | 0.5 |
| Carbon | 0 | 0.35365 | 0.93904 |
| Carbon | 0.5 | 0.35365 | 0.43904 |
| Carbon | 0.5 | 0.5 | 0 |
| Carbon | 0 | 0.5 | 0.5 |

TABLE XIII. Structural parameters of C-pw-TS. All units in [Å]. Atomic positions in fractional coordinates. See article for further details.

| | | | |
|---|---|---|---|
| $\|\vec{a}\|$ | 2.46115000 | 0.00000000 | 0.00000000 |
| $\|\vec{b}\|$ | 0.00000000 | 4.26283642 | 0.00000000 |
| $\|\vec{c}\|$ | 0.00000000 | 0.00000000 | 4.77969000 |
| Carbon | 0 | 0 | 0 |
| Carbon | 0 | 0 | 0.441024 |
| Carbon | 0.5 | 0.8333333333 | 0.5 |
| Carbon | 0.5 | 0.8333333333 | 0.941024 |
| Carbon | 0.5 | 0.5 | 0 |
| Carbon | 0.5 | 0.5 | 0.441024 |
| Carbon | 0 | 0.3333333333 | 0.5 |
| Carbon | 0 | 0.3333333333 | 0.941024 |

TABLE XIV. Structural parameters of G-ABC. All units in [Å]. Atomic positions in fractional coordinates. See article for further details.

| | | | |
|---|---|---|---|
| $\|\vec{a}\|$ | 2.44577000 | 0.00000000 | 0.00000000 |
| $\|\vec{b}\|$ | 0.00000000 | 4.23619790 | 0.00000000 |
| $\|\vec{c}\|$ | 0.00000000 | 1.41205938 | 6.58488117 |
| Carbon | 0.5 | 0.8333333333 | 0 |
| Carbon | 0 | 0.8333333333 | 0.5 |
| Carbon | 0 | 0 | 0 |
| Carbon | 0.5 | 0 | 0.5 |
| Carbon | 0 | 0.3333333333 | 0 |
| Carbon | 0.5 | 0.3333333333 | 0.5 |
| Carbon | 0.5 | 0.5 | 0 |
| Carbon | 0 | 0.5 | 0.5 |

TABLE XV. Structural parameters of G-AB. All units in [Å]. Atomic positions in fractional coordinates. See article for further details.

| | | | |
|---|---|---|---|
| $\|\vec{a}\|$ | 2.44582000 | 0.00000000 | 0.00000000 |
| $\|\vec{b}\|$ | 0.00000000 | 4.23628408 | 0.00000000 |
| $\|\vec{c}\|$ | 0.00000000 | 0.00000000 | 6.59022000 |
| Carbon | 0 | 0 | 0 |
| Carbon | 0 | 0 | 0.5 |
| Carbon | 0 | 0.333333 | 0 |
| Carbon | 0.5 | 0.1666666667 | 0.5 |
| Carbon | 0.5 | 0.5 | 0 |
| Carbon | 0.5 | 0.5 | 0.5 |
| Carbon | 0.5 | 0.833333 | 0 |
| Carbon | 0 | 0.6666666667 | 0.5 |

TABLE XVI. Structural parameters of G-AA. All units in [Å]. Atomic positions in fractional coordinates. See article for further details.

| | | | |
|---|---|---|---|
| $\|\vec{a}\|$ | 2.44549000 | 0.00000000 | 0.00000000 |
| $\|\vec{b}\|$ | 0.00000000 | 4.23570000 | 0.00000000 |
| $\|\vec{c}\|$ | 0.00000000 | 0.00000000 | 7.17071000 |
| Carbon | 0.5 | 0.5 | 0 |
| Carbon | 0.5 | 0.5 | 0.5 |
| Carbon | 0 | 0.3333333333 | 0.5 |
| Carbon | 0 | 0.3333333333 | 0 |
| Carbon | 0 | 0 | 0 |
| Carbon | 0 | 0 | 0.5 |
| Carbon | 0.5 | 0.8333333333 | 0.5 |
| Carbon | 0.5 | 0.8333333333 | 0 |

TABLE XVII. Structural parameters of $c$-D. All units in [Å]. Atomic positions in fractional coordinates. See article for further details.

| | | | |
|---|---|---|---|
| $\|\vec{a}\|$ | 2.49786000 | 0.00000000 | 0.00000000 |
| $\|\vec{b}\|$ | 0.00000000 | 4.32642043 | 0.00000000 |
| $\|\vec{c}\|$ | 0.00000000 | 1.44213268 | 4.07898175 |
| Carbon | 0.5 | 0.875 | 0.875 |
| Carbon | 0 | 0.875 | 0.375 |
| Carbon | 0 | 0 | 0 |
| Carbon | 0.499999 | 0 | 0.5 |
| Carbon | 0 | 0.375 | 0.875 |
| Carbon | 0.499999 | 0.375 | 0.375 |
| Carbon | 0.5 | 0.5 | 0 |
| Carbon | 0 | 0.5 | 0.5 |

TABLE XVIII. Structural parameters of $h$-D. All units in [Å]. Atomic positions in fractional coordinates. See article for further details.

| | | | |
|---|---|---|---|
| $\|\vec{a}\|$ | 2.48383000 | 0.00000000 | 0.00000000 |
| $\|\vec{b}\|$ | 0.00000000 | 4.30212062 | 0.00000000 |
| $\|\vec{c}\|$ | 0.00000000 | 0.00000000 | 4.13704000 |
| Carbon | 0 | 0 | 0 |
| Carbon | 0 | 0 | 0.37436 |
| Carbon | 0.5 | 0.8333333333 | 0.5 |
| Carbon | 0.5 | 0.8333333333 | 0.87436 |
| Carbon | 0.5 | 0.5 | 0 |
| Carbon | 0.5 | 0.5 | 0.37436 |
| Carbon | 0 | 0.3333333333 | 0.5 |
| Carbon | 0 | 0.3333333333 | 0.87436 |
